# Supplementary material for: Distributed In-Context Learning under Non-IID Among Clients
Source: arXiv:2408.00144 source file (2024-07-31)
Supplement: Supplementary file 1 [file 00_app.tex]

\appendix
\supptitle

This is the supplementary material for the \mytitle paper. Due to page limitations, we provide additional details as follows: (1) A detailed description of constructing non-IIDness in~\autoref{app:non_iid}, Following that, we outline the experimental setting of~\autoref{sec:motivation} in~\autoref{app:motive_exp_1}. In~\autoref{app:baseline} and~\autoref{app:exp_setting}, we describe the baselines of~\autoref{tab:main} and~\autoref{sec:exp}, respectively. Lastly, we summarize the method of constructing generated samples for privacy in~\autoref{app:paraphrase}.

\section{How we construct non-IIDness}
\label{app:non_iid}

Following \citet{li2022federated}, we use class number based non-IID partition in our experiment. For a dataset with overall $\Gamma$ classes, given hyperparameter class number $\gamma$ on each client, we randomly assign $\gamma$ classes from the overall $\Gamma$ classes for each client. Assuming that $C_1 \leq C$ clients are assigned with a specific class, we equally partition samples of this class into $C_1$ parts and assign one part to each of $C_1$ clients. We denote this non-IID partition with the class number $\gamma$ on each client as \texttt{noniid-\#label=$\gamma$}.

\section{Motivation Experimental Settings}
\label{app:motive_exp_1}

\myparagraph{Non-IIDness performance drop experiment.}
For this experiment, we use SST5, Amazon, Yelp, Yahoo, and AGNews. And the non-iid settings are dsecribed in~\autoref{tab:motivation_setting}.

\begin{table}[h]
    \centering
    \begin{tabular}{cccc}
    \thickhline
        Dataset & ICE size $k$ & \#Clients & Partition \\\hline
        SST-5   & 32    & 8 & \texttt{noniid-\#label=1}\\
        Amazon  & 16    & 8 & \texttt{noniid-\#label=1}\\
        Yahoo   & 16    & 8 & \texttt{noniid-\#label=2}\\
        AGNews  & 16    & 4 & \texttt{noniid-\#label=1}\\
        Yelp    & 4     & 2 & \texttt{noniid-\#label=3}\\
    \thickhline
    \end{tabular}
    \caption{Experimental setup for obtaining the motivation.}
    \label{tab:motivation_setting}
\end{table}

% \begin{itemize}
%     \item SST5: centralized with 32 ICEs; 8 clients IID with 32 ICEs; 8 clients \texttt{noniid-\#label=1} with 32 ICEs
%     \item Amazon: centralized with 16 ICEs; 8 clients IID with 16 ICEs; 8 clients \texttt{noniid-\#label=1} with 16 ICEs
%     \item Yelp: centralized with 4 ICEs; 2 clients IID with 4 ICEs; 2 clients \texttt{noniid-\#label=3} with 4 ICEs
%     \item Yahoo: centralized with 16 ICEs; 8 clients IID with 16 ICEs; 8 clients \texttt{noniid-\#label=2} with 16 ICEs
%     \item AGNews: centralized with 16 ICEs; 4 clients IID with 16 ICEs; 4 clients \texttt{noniid-\#label=1} with 16 ICEs
% \end{itemize}

\myparagraph{t-SNE analysis of per-client budget experiment.} For extracting t-SNE figure, we utilized the following experimental setting~\autoref{tab:motivation_setting_tsne}

\begin{table}[h]
    \centering
    \begin{tabular}{cccc}
    \thickhline
        Dataset & ICE size $k$ & \#Clients & Partition \\\hline
        SST-5   & 32    & 4 & \texttt{noniid-\#label=2}\\
        Yelp    & 8     & 2 & \texttt{noniid-\#label=3}\\
    \thickhline
    \end{tabular}
    \caption{Experimental setup for obtaining the motivation.}
    \label{tab:motivation_setting_tsne}
\end{table}

% \begin{itemize}
%     \item SST5: 4 clients \texttt{noniid-\#label=2} with 32 ICEs, the oracle budgets construction uses local budget as 32 for each client
%     \item Yelp: 2 clients \texttt{noniid-\#label=3} with 8 ICEs, the oracle budgets construction uses local budget as 16 for each client
% \end{itemize} \newpage
\section{Baseline Details}
\label{app:baseline}

\myparagraph{Proxy-only.} We randomly select samples from the original test set to construct the proxy set on the server side and use the remaining test set as the true test set. When performing the ICL process, the server directly retrieves ICEs from the proxy set rather than from the training set.
For SST5, MR, and Subj, we randomly select 500 samples from the test set to be the proxy set.
For Amazon, Yelp, Yahoo, and Agnews, we randomly select 750 samples from the test set to be the proxy set. Also, since the proxy set is already on the server side, there will be no privacy issues during communication between clients and the server. Thus, we don't generate samples to protect privacy and directly use the original samples in the proxy set for ICL. 

\myparagraph{Singleton.} This baseline is for if the whole ICE set is constructed only using single client's local dataset. We randomly select one client from $C$ clients, and perform local retrieval with $k_c=k$ budget. Then, the server uses this locally retrieved ICE set for LLM inference. We report the average accuracy over all clients.

\myparagraph{Social learning.} This algorithm~\cite{mohtashami2023social} is the first paper that considers the distributed ICL, but it only considers the IID setting. Since the authors didn't release the source code, we implemented it on our own. In our implementation, given server-side ICE number as $k$, each local client $c$ performs local top-$\left\lceil \frac{k}{C} \right\rceil$ retrieval and sends retrieved ICEs to the server. The server then performs a random selection from $k$ ICEs to construct an ICE set with $k$ samples and feed this ICE set into LLM for inference. 

\myparagraph{Uniform-budget.} We equally assign a local budget to each client. Assume the ICE number fed to server-side LLM for inference is $k$, then each client's local budget is $\left\lceil\frac{k}{C}\right\rceil$, where $C$ is the number of clients. On server-side aggregation, we use \texttt{reorder} method as default.

\myparagraph{Random-budget.} We randomly assign a local budget to each client with the constraint that the overall local budget over $C$ clients is $k$, where $k$ is the ICE number fed to server-side LLM. On server-side aggregation, we use \texttt{reorder} method as default.

\myparagraph{$\infty$-budget.} The most inefficient way to do distributed non-IID ICL is to allow $\infty$-budget on each client, that is, sending all samples to the server side. Then, the system performs centralized retrieval on the collected dataset to obtain top-$k$ ICEs and feed them into LLM for inference. 
 
\section{Experimental Setting}
\label{app:exp_setting}

\myparagraph{Dataset Explanation.}
In this study, we utilized seven text classification tasks: four for sentiment analysis, two for topic classification, and one for subjectivity classification. The dataset statistics are presented in~\autoref{tab:dataset_statistics}. 

\begin{table}[h]
    \centering
    \resizebox{0.5\linewidth}{!}{
    \begin{tabular}{cccccc}
    \thickhline
        Dataset     & Type          & Training      & Test          & Class\\ \hline
        SST-5       & Sentiment     & 8.534         & 2,210         & 5          \\
        Amazon      & Sentiment     & 30,000        & 3,000         & 5          \\
        Yelp        & Sentiment     & 30,000        & 3,000         & 2          \\
        MR          & Sentiment     & 8,662         & 2,000         & 2          \\
        Yahoo       & Topic         & 29,150        & 3,000         & 10         \\
        AGNews      & Topic         & 29,914        & 3,000         & 4          \\
        Subj        & Subjectivity  & 8,000         & 2,000         & 2          \\
    \thickhline
    \end{tabular}}
    \caption{The statistics of the datasets used.}
    \label{tab:dataset_statistics}
\end{table}
\noindent
Given that the input instruction prompt can notably influence performance, we detail the prompts used for each dataset in~\autoref{tab:prompt}. It is in the last page since prompts have long length. We follow the prompt settings described in~\cite{li2023unified} and use the dataset uploaded by the paper's author, available at \url{https://huggingface.co/KaiLv}.

\myparagraph{ICE number for LLM inference.} Given an LLM, different datasets show different preferences on the choice of ICE number, \ie $k$, used in ICL inference for better performance. For algorithms using ICL (except Zero-shot), SST5, MR, and Subj use 32 ICEs for server-side LLM inference; Amazon uses 8 ICEs for server-side LLM inference; Yelp, Yahoo, and Agnews use 4 ICEs for server-side LLM inference.

\myparagraph{Non-IID Setting.} To keep similar non-IIDness levels across different datasets, we follow~\autoref{tab:app_noniid} as non-IID hyper-parameters for each dataset.

\myparagraph{Hyper-parameters for our methods.} For the main table results, the generated dataset results, and the different LLM architecture results, the hyper-parameters are shown in~\autoref{tab:app_main_hyper}, \autoref{tab:app_gen_hyper} and \autoref{tab:app_LLM_arch_hyper}, respectively. For the training of the budget model, we use 800 epochs, with a learning rate range $\{0.01, 0.003\}$ and a batch size of 8.

\myparagraph{Multi-layer perceptron for budget allocator.}
We use the three-layer perceptron on top of the encoder $\mc{E}$. The \code{torch} pseudo code is as follows:
\begin{shaded}
\noindent
\code{class SMLP(nn.Module):}\\
\code{\phantom{aaaa}def \_\_init\_\_(self, width=300, num\_classes=10, data\_shape=(768,)):}\\
\code{\phantom{aaaa}\phantom{aaaa}super().\_\_init\_\_()}\\
\code{\phantom{aaaa}\phantom{aaaa}self.flat = nn.Flatten()}\\
\code{\phantom{aaaa}\phantom{aaaa}self.l1 = nn.Linear(np.prod(data\_shape), width)}\\
\code{\phantom{aaaa}\phantom{aaaa}self.relu = nn.ReLU()}\\
\code{\phantom{aaaa}\phantom{aaaa}self.l2 = nn.Linear(width, width)}\\
\code{\phantom{aaaa}\phantom{aaaa}self.l3 = nn.Linear(width, num\_classes)}\\
\code{}\\
\code{\phantom{aaaa}def forward(self, x):}\\
\code{\phantom{aaaa}\phantom{aaaa}x = self.flat(x)}\\
\code{\phantom{aaaa}\phantom{aaaa}x = self.l1(x)}\\
\code{\phantom{aaaa}\phantom{aaaa}x = self.relu(x)}\\
\code{\phantom{aaaa}\phantom{aaaa}x = self.l2(x)}\\
\code{\phantom{aaaa}\phantom{aaaa}x = self.relu(x)}\\
\code{\phantom{aaaa}\phantom{aaaa}x = self.l3(x)}\\
\code{\phantom{aaaa}\phantom{aaaa}x = F.softmax(x)}\\
\code{\phantom{aaaa}\phantom{aaaa}return x}
\end{shaded}

\begin{table}[h]
    \centering
    \begin{tabular}{ccc}
    \thickhline
        Dataset & \#Clients  & Partition \\\hline
        SST-5   & 4 & \texttt{noniid-\#label=2}\\
        Amazon  & 2 & \texttt{noniid-\#label=3}\\
        Yelp    & 2 & \texttt{noniid-\#label=3}\\
        MR      & 4 & \texttt{noniid-\#label=1}\\
        Yahoo   & 2 & \texttt{noniid-\#label=5}\\
        AGNews  & 2 & \texttt{noniid-\#label=2}\\
        Subj    & 4 & \texttt{noniid-\#label=1}\\
        \thickhline
    \end{tabular}
    \caption{Non-IID setting}
    \label{tab:app_noniid}
\end{table}
% \begin{itemize}
%     \item SST5: 4 clients with \texttt{noniid-\#label=2}
%     \item Amazon: 2 clients with \texttt{noniid-\#label=3}
%     \item Yelp: 2 clients with \texttt{noniid-\#label=3}
%     \item MR: 4 clients with \texttt{noniid-\#label=1}
%     \item Yahoo: 2 clients with \texttt{noniid-\#label=5}
%     \item Agnews: 2 clients with \texttt{noniid-\#label=2}
%     \item Subj: 4 clients with \texttt{noniid-\#label=1}
% \end{itemize}

\begin{table}[h]
    \centering
    \begin{tabular}{ccccc}
    \thickhline
        Dataset & ProxySetSize  & $\delta$ & $\alpha$ & QuantRatio  \\\hline
        SST-5   & 500 & 3 
                & 0 & 0.5  \\
        Amazon  & 750 & 2 
                & 0 & 0.5\\
        Yelp    & 750 & 2 
                & 2 & 0.5 \\
        MR      & 500 & 3 
                & 0 & 0.5 \\
        Yahoo   & 750 & 2 
                & 2 & 0.5 \\
        AGNews  & 750 & 2 
                & 2  & 0.5 \\
        Subj    & 500 & 3 
                & 0  & 0.3 \\
        \thickhline
    \end{tabular}
    \caption{Hyper-parameters of our methods used in the main table}
    \label{tab:app_main_hyper}
\end{table}

\begin{table}[h]
    \centering
    \begin{tabular}{ccccc}
    \thickhline
        Dataset  %& \texttt{learning\_rate} 
        & ProxySetSize  & $\delta$ & $\alpha$ & QuantRatio \\\hline
        SST-5 %&   
        & 500 & 3 
                & 4 & 0.5 \\
        Yelp %&   
        & 750 & 3 
                & 0 & 0.5 \\
        Subj %& 0.003  
        & 500 & 3 
                & 0 & 0.3\\
        \thickhline
    \end{tabular}
    \caption{Hyper-parameters of our methods used for the generated query and training samples experiment}
    \label{tab:app_gen_hyper}
\end{table}

\begin{table}[h]
    \centering
    \begin{tabular}{ccccc}
    \thickhline
        Model %& \texttt{learning\_rate} 
        & ProxySetSize  & $\delta$ & $\alpha$ & QuantRatio \\\hline
        GPT-Neo-1.3B  %&  0.003  
        & 500 & 3   & 0 & 0.3 \\
        GPT-Neo-2.7B  %&  0.003  
        & 500 & 3   & 0 & 0.3 \\
        % Gemma-2B      &  0.003  & 500 & 3   & 0 & 0.3 \\
        Llama-2-7B    %&  0.003  
        & 500 & 3   & 0 & 0.3 \\
        \thickhline
    \end{tabular}
    \caption{Hyper-parameters of our methods used for different LLM architectures experiment on Subj}
    \label{tab:app_LLM_arch_hyper}
\end{table}

 \newpage
\section{Generate paraphrased question}
\label{app:paraphrase}

To generate the paraphrased query and response, we use the following instruction.
\begin{shaded}
\noindent
Please paraphrase the original sentence. Original sentence: \{In-context example\} Paraphrase sentence: \{Paraphrased sentence\}
\end{shaded}
\noindent
Here is an example of input for the rephrasing LLM using the SST-5 dataset.
\begin{shaded}
\noindent
Please paraphrase the original sentence. Original sentence: "a stirring, funny and finally transporting re-imagining of beauty and the beast and 1930s horror films" Paraphrased sentence: A captivating, humorous, and ultimately uplifting reinterpretation of Beauty and the Beast combined with 1930s horror films. 
Please paraphrase the original sentence. Original sentence: "jonathan parker 's bartleby should have been the be-all-end-all of the modern-office anomie films" Paraphrased sentence: Jonathan Parker's "Bartleby" had the potential to be the definitive film capturing the sense of alienation in modern office settings. 
Please paraphrase the original sentence. Original sentence: "a fan film that for the uninitiated plays better on video with the sound turned down" Paraphrased sentence: A fan film that, for those not familiar with the source material, is more enjoyable when watched with the sound turned off. 
Please paraphrase the original sentence. Original sentence: "apparently reassembled from the cutting-room floor of any given daytime soap" Paraphrased sentence: It appears to be pieced together from the outtakes of any given daytime soap opera. 
Please paraphrase the original sentence. Original sentence: "{}" Paraphrased sentence:
\end{shaded}

\noindent
Our paraphrased examples are summarized as follows.

\begin{table}[h]
    \centering
    \begin{tabular}{p{7.3cm}p{7.3cm}}
    \thickhline
        Original & Paraphrased \\ \hline
        a turgid little history lesson , humourless and dull  &
        A dry and tedious history lesson that is devoid of humour or interest.  \\ 
        not so much a movie as a picture book for the big screen .&
        The movie is more of a picture book than a full-fledged movie for the big screen.\\ 
        now it 's just tired .  &
        It is now simply outdated. \\  
    \thickhline
    \end{tabular}
    \caption{Paraphrased examples of SST-5 dataset}
    \label{tab:my_label}
\end{table}

\begin{table}[h]
    \centering
    \begin{tabular}{p{7.3cm}p{7.3cm}}
    \thickhline
        Original & Paraphrased \\ \hline
        for all the wit and hoopla , festival in cannes offers rare insight into the structure of relationships .&
        Festival in Cannes offers rare insight into the structure of relationships.\\ 
        eldom has a movie so closely matched the spirit of a man and his work .&
        A movie seldom has a movie so closely matched the spirit of a man and his work.\\ 
        those of you who are not an eighth grade girl will most likely doze off during this one . &
        8th graders and younger will most likely doze off during this one.\\  
    \thickhline
    \end{tabular}
    \caption{Paraphrased examples of Subj dataset}
    \label{tab:my_label}
\end{table}

\begin{table}[h]
    \centering
    \begin{tabular}{p{7.3cm}p{7.3cm}}
    \thickhline
        Original & Paraphrased \\ \hline
        A friend of mine suggested we go here today before our movie. I was planning on suggesting another place, but she got their early and got a table DARN!I don't hate Red Robin...I think I avoid it because I am not a big fan of hamburgers. Seems like more of a place for straight guys and kids if you ask me, but my experience today wasn't to bad.Our waiter was really nice however I think that may have been a result of my push up bra.Ordered the Crispy Chicken Salad which also had hard boiled egg, bacon, and veggies and was very good. I'll probably get that again next time someone drags me here. Get it with that Italian dressing. Yummy! My friend ordered us onion rings as an appetizer I hate onions, but those were goood! Not my first choice but good crowd pleaser with more decent food than most chains.&
        I was considering going to Red Robin with a friend, but I decided to go somewhere else instead. I was not a big fan of hamburgers, but I was drawn to Red Robin because of the free tastings. I was pleasantly surprised by the friendliness of the staff, especially the waiter who was very attentive and helpful. I ordered the Crispy Chicken Salad, which was very good. I'll probably go back there next time someone drags me there. \\ 
        Huge rooms. Soft towels. Comfortable bed with tons of pillows. Three things that make me happy when I'm traveling. What's wrong with this place, then? First of all, the location is central to nothing aside from the mall which houses several chain restaurants. Second, the staff could not care less about pretty much anything. While the woman who checked us in was helpful and friendly, that was the end of that. Despite requesting my Hilton status "amenities" (just a package of snacks and water...not much), I never received it. I was also charged \$30 for internet when I shouldn't have paid a thing (got the bill corrected at check out). And housekeeping didn't leave enough towels or replace the water. Considering we paid over 200 a night, the blase attitude of the staff is very disappointing. &
        3 things that make me happy when I travel are: spacious rooms, friendly staff, and a comfortable bed with lots of pillows. However, the location is inconvenient, the staff is indifferent, and the amenities are subpar.\\ 
        You can either pay \$5.50 for 3-day movie rentals or get a \$40 membership and pay \$2 for 3-day/\$3 for 7-day rentals. They also offer 2-for-1 movies for students on Tuesday and Thursday. The reason I give 3 stars is because that deal isn't valid for people with memberships!? I learnt this 30 seconds after paying for a membership. I'm a student and could have paid \$2.75 for movies twice a week. Instead I paid \$40 (way too much) for a membership to pay .75 cents less than the other students. Good movie selection and shop but don't fall for their rip off of a membership unless you rent daily. &
        3-day movie rentals cost either \$5.50 or \$40 for a membership. They offer a deal for students on Tuesdays and Thursdays, but it's not valid for those with memberships.\\ 
        
    \thickhline
    \end{tabular}
    \caption{Paraphrased examples of Yelp dataset}
    \label{tab:my_label}
\end{table} \newpage

\begin{table}[h]
\centering
\resizebox{0.95\linewidth}{!}{
\begin{tabular}{c|p{3cm}|p{3.1cm}|c|p{6cm}}
\thickhline
Dataset & Prompt & Label & Label Template & Example\\ \hline
AGNews   & Topic of the text: & \{World, Sports, Business, Technology \} & Topic: \textbf{\textit{Label}} & \textcolor{blue}{REDMOND, Wash. - Microsoft Corp. and cable television provider Comcast Corp. said Monday they would begin deploying set-top boxes powered by Microsoft software starting next week. \textbackslash n Topic: Business \textbackslash\textbackslash ...}\textcolor{red}{Oil demand is rising faster than predicted this year as OPEC pumps more low-quality oil in a failed bid to reduce record prices, according to International Energy Agency, an adviser to 26 industrialized nations. \textbackslash n Topic:}  \\ \hline

MR   & Sentiment of the sentence: & \{great, terrible\} & It was \textbf{\textit{Label}} & \textcolor{blue}{"Analyze That" is one of those crass, contrived sequels that not only fails on its own but makes you second-guess your affection for the original. \textbackslash n It was terrible ...}\textcolor{red}{about the only thing to give the movie points for is bravado—to take an entirely stale concept and push it through the audience's meat grinder one more time.\textbackslash n It was }  \\ \hline

SST-5   & Sentiment of the sentence: & \{great, good, okay, bad, terrible\} & It was \textbf{\textit{Label}} & \textcolor{blue}{a strong, funny, and finally transporting re-imagining of Beauty and the Beast and 1930s horror films \textbackslash n It was great ...}\textcolor{red}{no movement, no yuks, not much of anything. \textbackslash n It was}  \\ \hline

Subj   & Subjectivity of the sentence: & \{subjective, objective\} & It's \textbf{\textit{Label}} & \textcolor{blue}{gangs, despite the gravity of its subject matter, is often as fun to watch as a good spaghetti western. \textbackslash n It's subjective ...}\textcolor{red}{smart and alert, Thirteen Conversations About One Thing is a small gem. \textbackslash n It's}  \\ \hline

Amazon    & Sentiment of the sentence: & \{great, good, okay, bad, terrible\} & It was \textbf{\textit{Label}} 
& \textcolor{blue}{Love the originality of this music. Because she is ever-changing, Madonna is never boring. "Music" makes you want to dance - totally energizing! Wish the "Music" video was half as impressive as this work of art. ...}
\textcolor{red}{The case for the DVDs were a bit damaged. The damage did not compromise the DVDs, ... \textbackslash n It's}  \\ \hline

Yelp   & Subjectivity of the sentence: & \{subjective, objective\} & It's \textbf{\textit{Label}} & \textcolor{blue}{My family visited ceasars palace and ate here. Our waiting time was only ten minutes despite all the people. Our server was the best. He recommended several great dishes. The food was higher than our expections....}\textcolor{red}{his place is great. The staff is really friendly and the chile verde burrito is fantastic. You know a ...  \textbackslash n It's}  \\ \hline

Yahoo   & Topic of the sentence & \{Society \& Culture, Science \& Mathematics, Health, Education \& Reference, Computers \& Internet, Sports, Business \& Finance, Entertainment \& Music, Family \& Relationships, Politics \& Government\} & It's \textbf{\textit{Label}} & \textcolor{blue}{who sang message in a bottle? Answer: Sting (the Police) ...}\textcolor{red}{Neuroscience Question? Answer: no it is callef motor neuroprostheses. \textbackslash n Topic: }  \\
\thickhline
\end{tabular}}
\caption{Prompt and instructions used for each dataset. We denote \textcolor{blue}{examples} in blue and \textcolor{red}{queries} in red.}
\label{tab:prompt}
\end{table}
