# Supplementary material for: Distributed In-Context Learning under Non-IID Among Clients
Source: arXiv:2408.00144 source file (2024-07-31)
Supplement: Supplementary file 2 [file 01_non_iid.tex]

\section{How we construct non-IIDness}
\label{app:non_iid}

Following \citet{li2022federated}, we use class number based non-IID partition in our experiment. For a dataset with overall $\Gamma$ classes, given hyperparameter class number $\gamma$ on each client, we randomly assign $\gamma$ classes from the overall $\Gamma$ classes for each client. Assuming that $C_1 \leq C$ clients are assigned with a specific class, we equally partition samples of this class into $C_1$ parts and assign one part to each of $C_1$ clients. We denote this non-IID partition with the class number $\gamma$ on each client as \texttt{noniid-\#label=$\gamma$}.
