# Supplementary material for: Distributed In-Context Learning under Non-IID Among Clients
Source: arXiv:2408.00144 source file (2024-07-31)
Supplement: Supplementary file 3 [file 02_motive_exp_1.tex]

\section{Motivation Experimental Settings}
\label{app:motive_exp_1}

\myparagraph{Non-IIDness performance drop experiment.}
For this experiment, we use SST5, Amazon, Yelp, Yahoo, and AGNews. And the non-iid settings are dsecribed in~\autoref{tab:motivation_setting}.

\begin{table}[h]
    \centering
    \begin{tabular}{cccc}
    \thickhline
        Dataset & ICE size $k$ & \#Clients & Partition \\\hline
        SST-5   & 32    & 8 & \texttt{noniid-\#label=1}\\
        Amazon  & 16    & 8 & \texttt{noniid-\#label=1}\\
        Yahoo   & 16    & 8 & \texttt{noniid-\#label=2}\\
        AGNews  & 16    & 4 & \texttt{noniid-\#label=1}\\
        Yelp    & 4     & 2 & \texttt{noniid-\#label=3}\\
    \thickhline
    \end{tabular}
    \caption{Experimental setup for obtaining the motivation.}
    \label{tab:motivation_setting}
\end{table}

% \begin{itemize}
%     \item SST5: centralized with 32 ICEs; 8 clients IID with 32 ICEs; 8 clients \texttt{noniid-\#label=1} with 32 ICEs
%     \item Amazon: centralized with 16 ICEs; 8 clients IID with 16 ICEs; 8 clients \texttt{noniid-\#label=1} with 16 ICEs
%     \item Yelp: centralized with 4 ICEs; 2 clients IID with 4 ICEs; 2 clients \texttt{noniid-\#label=3} with 4 ICEs
%     \item Yahoo: centralized with 16 ICEs; 8 clients IID with 16 ICEs; 8 clients \texttt{noniid-\#label=2} with 16 ICEs
%     \item AGNews: centralized with 16 ICEs; 4 clients IID with 16 ICEs; 4 clients \texttt{noniid-\#label=1} with 16 ICEs
% \end{itemize}

\myparagraph{t-SNE analysis of per-client budget experiment.} For extracting t-SNE figure, we utilized the following experimental setting~\autoref{tab:motivation_setting_tsne}

\begin{table}[h]
    \centering
    \begin{tabular}{cccc}
    \thickhline
        Dataset & ICE size $k$ & \#Clients & Partition \\\hline
        SST-5   & 32    & 4 & \texttt{noniid-\#label=2}\\
        Yelp    & 8     & 2 & \texttt{noniid-\#label=3}\\
    \thickhline
    \end{tabular}
    \caption{Experimental setup for obtaining the motivation.}
    \label{tab:motivation_setting_tsne}
\end{table}

% \begin{itemize}
%     \item SST5: 4 clients \texttt{noniid-\#label=2} with 32 ICEs, the oracle budgets construction uses local budget as 32 for each client
%     \item Yelp: 2 clients \texttt{noniid-\#label=3} with 8 ICEs, the oracle budgets construction uses local budget as 16 for each client
% \end{itemize}
