# Supplementary material for: Distributed In-Context Learning under Non-IID Among Clients
Source: arXiv:2408.00144 source file (2024-07-31)
Supplement: Supplementary file 4 [file 03_baseline.tex]

\section{Baseline Details}
\label{app:baseline}

\myparagraph{Proxy-only.} We randomly select samples from the original test set to construct the proxy set on the server side and use the remaining test set as the true test set. When performing the ICL process, the server directly retrieves ICEs from the proxy set rather than from the training set.
For SST5, MR, and Subj, we randomly select 500 samples from the test set to be the proxy set.
For Amazon, Yelp, Yahoo, and Agnews, we randomly select 750 samples from the test set to be the proxy set. Also, since the proxy set is already on the server side, there will be no privacy issues during communication between clients and the server. Thus, we don't generate samples to protect privacy and directly use the original samples in the proxy set for ICL. 

\myparagraph{Singleton.} This baseline is for if the whole ICE set is constructed only using single client's local dataset. We randomly select one client from $C$ clients, and perform local retrieval with $k_c=k$ budget. Then, the server uses this locally retrieved ICE set for LLM inference. We report the average accuracy over all clients.

\myparagraph{Social learning.} This algorithm~\cite{mohtashami2023social} is the first paper that considers the distributed ICL, but it only considers the IID setting. Since the authors didn't release the source code, we implemented it on our own. In our implementation, given server-side ICE number as $k$, each local client $c$ performs local top-$\left\lceil \frac{k}{C} \right\rceil$ retrieval and sends retrieved ICEs to the server. The server then performs a random selection from $k$ ICEs to construct an ICE set with $k$ samples and feed this ICE set into LLM for inference. 

\myparagraph{Uniform-budget.} We equally assign a local budget to each client. Assume the ICE number fed to server-side LLM for inference is $k$, then each client's local budget is $\left\lceil\frac{k}{C}\right\rceil$, where $C$ is the number of clients. On server-side aggregation, we use \texttt{reorder} method as default.

\myparagraph{Random-budget.} We randomly assign a local budget to each client with the constraint that the overall local budget over $C$ clients is $k$, where $k$ is the ICE number fed to server-side LLM. On server-side aggregation, we use \texttt{reorder} method as default.

\myparagraph{$\infty$-budget.} The most inefficient way to do distributed non-IID ICL is to allow $\infty$-budget on each client, that is, sending all samples to the server side. Then, the system performs centralized retrieval on the collected dataset to obtain top-$k$ ICEs and feed them into LLM for inference.
