# Supplementary material for: Distributed In-Context Learning under Non-IID Among Clients
Source: arXiv:2408.00144 source file (2024-07-31)
Supplement: Supplementary file 5 [file 04_exp_setting.tex]

\section{Experimental Setting}
\label{app:exp_setting}

\myparagraph{Dataset Explanation.}
In this study, we utilized seven text classification tasks: four for sentiment analysis, two for topic classification, and one for subjectivity classification. The dataset statistics are presented in~\autoref{tab:dataset_statistics}. 

\begin{table}[h]
    \centering
    \resizebox{0.5\linewidth}{!}{
    \begin{tabular}{cccccc}
    \thickhline
        Dataset     & Type          & Training      & Test          & Class\\ \hline
        SST-5       & Sentiment     & 8.534         & 2,210         & 5          \\
        Amazon      & Sentiment     & 30,000        & 3,000         & 5          \\
        Yelp        & Sentiment     & 30,000        & 3,000         & 2          \\
        MR          & Sentiment     & 8,662         & 2,000         & 2          \\
        Yahoo       & Topic         & 29,150        & 3,000         & 10         \\
        AGNews      & Topic         & 29,914        & 3,000         & 4          \\
        Subj        & Subjectivity  & 8,000         & 2,000         & 2          \\
    \thickhline
    \end{tabular}}
    \caption{The statistics of the datasets used.}
    \label{tab:dataset_statistics}
\end{table}
\noindent
Given that the input instruction prompt can notably influence performance, we detail the prompts used for each dataset in~\autoref{tab:prompt}. It is in the last page since prompts have long length. We follow the prompt settings described in~\cite{li2023unified} and use the dataset uploaded by the paper's author, available at \url{https://huggingface.co/KaiLv}.

\myparagraph{ICE number for LLM inference.} Given an LLM, different datasets show different preferences on the choice of ICE number, \ie $k$, used in ICL inference for better performance. For algorithms using ICL (except Zero-shot), SST5, MR, and Subj use 32 ICEs for server-side LLM inference; Amazon uses 8 ICEs for server-side LLM inference; Yelp, Yahoo, and Agnews use 4 ICEs for server-side LLM inference.

\myparagraph{Non-IID Setting.} To keep similar non-IIDness levels across different datasets, we follow~\autoref{tab:app_noniid} as non-IID hyper-parameters for each dataset.

\myparagraph{Hyper-parameters for our methods.} For the main table results, the generated dataset results, and the different LLM architecture results, the hyper-parameters are shown in~\autoref{tab:app_main_hyper}, \autoref{tab:app_gen_hyper} and \autoref{tab:app_LLM_arch_hyper}, respectively. For the training of the budget model, we use 800 epochs, with a learning rate range $\{0.01, 0.003\}$ and a batch size of 8.

\myparagraph{Multi-layer perceptron for budget allocator.}
We use the three-layer perceptron on top of the encoder $\mc{E}$. The \code{torch} pseudo code is as follows:
\begin{shaded}
\noindent
\code{class SMLP(nn.Module):}\\
\code{\phantom{aaaa}def \_\_init\_\_(self, width=300, num\_classes=10, data\_shape=(768,)):}\\
\code{\phantom{aaaa}\phantom{aaaa}super().\_\_init\_\_()}\\
\code{\phantom{aaaa}\phantom{aaaa}self.flat = nn.Flatten()}\\
\code{\phantom{aaaa}\phantom{aaaa}self.l1 = nn.Linear(np.prod(data\_shape), width)}\\
\code{\phantom{aaaa}\phantom{aaaa}self.relu = nn.ReLU()}\\
\code{\phantom{aaaa}\phantom{aaaa}self.l2 = nn.Linear(width, width)}\\
\code{\phantom{aaaa}\phantom{aaaa}self.l3 = nn.Linear(width, num\_classes)}\\
\code{}\\
\code{\phantom{aaaa}def forward(self, x):}\\
\code{\phantom{aaaa}\phantom{aaaa}x = self.flat(x)}\\
\code{\phantom{aaaa}\phantom{aaaa}x = self.l1(x)}\\
\code{\phantom{aaaa}\phantom{aaaa}x = self.relu(x)}\\
\code{\phantom{aaaa}\phantom{aaaa}x = self.l2(x)}\\
\code{\phantom{aaaa}\phantom{aaaa}x = self.relu(x)}\\
\code{\phantom{aaaa}\phantom{aaaa}x = self.l3(x)}\\
\code{\phantom{aaaa}\phantom{aaaa}x = F.softmax(x)}\\
\code{\phantom{aaaa}\phantom{aaaa}return x}
\end{shaded}

\begin{table}[h]
    \centering
    \begin{tabular}{ccc}
    \thickhline
        Dataset & \#Clients  & Partition \\\hline
        SST-5   & 4 & \texttt{noniid-\#label=2}\\
        Amazon  & 2 & \texttt{noniid-\#label=3}\\
        Yelp    & 2 & \texttt{noniid-\#label=3}\\
        MR      & 4 & \texttt{noniid-\#label=1}\\
        Yahoo   & 2 & \texttt{noniid-\#label=5}\\
        AGNews  & 2 & \texttt{noniid-\#label=2}\\
        Subj    & 4 & \texttt{noniid-\#label=1}\\
        \thickhline
    \end{tabular}
    \caption{Non-IID setting}
    \label{tab:app_noniid}
\end{table}
% \begin{itemize}
%     \item SST5: 4 clients with \texttt{noniid-\#label=2}
%     \item Amazon: 2 clients with \texttt{noniid-\#label=3}
%     \item Yelp: 2 clients with \texttt{noniid-\#label=3}
%     \item MR: 4 clients with \texttt{noniid-\#label=1}
%     \item Yahoo: 2 clients with \texttt{noniid-\#label=5}
%     \item Agnews: 2 clients with \texttt{noniid-\#label=2}
%     \item Subj: 4 clients with \texttt{noniid-\#label=1}
% \end{itemize}

\begin{table}[h]
    \centering
    \begin{tabular}{ccccc}
    \thickhline
        Dataset & ProxySetSize  & $\delta$ & $\alpha$ & QuantRatio  \\\hline
        SST-5   & 500 & 3 
                & 0 & 0.5  \\
        Amazon  & 750 & 2 
                & 0 & 0.5\\
        Yelp    & 750 & 2 
                & 2 & 0.5 \\
        MR      & 500 & 3 
                & 0 & 0.5 \\
        Yahoo   & 750 & 2 
                & 2 & 0.5 \\
        AGNews  & 750 & 2 
                & 2  & 0.5 \\
        Subj    & 500 & 3 
                & 0  & 0.3 \\
        \thickhline
    \end{tabular}
    \caption{Hyper-parameters of our methods used in the main table}
    \label{tab:app_main_hyper}
\end{table}

\begin{table}[h]
    \centering
    \begin{tabular}{ccccc}
    \thickhline
        Dataset  %& \texttt{learning\_rate} 
        & ProxySetSize  & $\delta$ & $\alpha$ & QuantRatio \\\hline
        SST-5 %&   
        & 500 & 3 
                & 4 & 0.5 \\
        Yelp %&   
        & 750 & 3 
                & 0 & 0.5 \\
        Subj %& 0.003  
        & 500 & 3 
                & 0 & 0.3\\
        \thickhline
    \end{tabular}
    \caption{Hyper-parameters of our methods used for the generated query and training samples experiment}
    \label{tab:app_gen_hyper}
\end{table}

\begin{table}[h]
    \centering
    \begin{tabular}{ccccc}
    \thickhline
        Model %& \texttt{learning\_rate} 
        & ProxySetSize  & $\delta$ & $\alpha$ & QuantRatio \\\hline
        GPT-Neo-1.3B  %&  0.003  
        & 500 & 3   & 0 & 0.3 \\
        GPT-Neo-2.7B  %&  0.003  
        & 500 & 3   & 0 & 0.3 \\
        % Gemma-2B      &  0.003  & 500 & 3   & 0 & 0.3 \\
        Llama-2-7B    %&  0.003  
        & 500 & 3   & 0 & 0.3 \\
        \thickhline
    \end{tabular}
    \caption{Hyper-parameters of our methods used for different LLM architectures experiment on Subj}
    \label{tab:app_LLM_arch_hyper}
\end{table}
