# Supplementary material for: Distributed In-Context Learning under Non-IID Among Clients
Source: arXiv:2408.00144 source file (2024-07-31)
Supplement: Supplementary file 6 [file 05_paraphrase.tex]

\section{Generate paraphrased question}
\label{app:paraphrase}

To generate the paraphrased query and response, we use the following instruction.
\begin{shaded}
\noindent
Please paraphrase the original sentence. Original sentence: \{In-context example\} Paraphrase sentence: \{Paraphrased sentence\}
\end{shaded}
\noindent
Here is an example of input for the rephrasing LLM using the SST-5 dataset.
\begin{shaded}
\noindent
Please paraphrase the original sentence. Original sentence: "a stirring, funny and finally transporting re-imagining of beauty and the beast and 1930s horror films" Paraphrased sentence: A captivating, humorous, and ultimately uplifting reinterpretation of Beauty and the Beast combined with 1930s horror films. 
Please paraphrase the original sentence. Original sentence: "jonathan parker 's bartleby should have been the be-all-end-all of the modern-office anomie films" Paraphrased sentence: Jonathan Parker's "Bartleby" had the potential to be the definitive film capturing the sense of alienation in modern office settings. 
Please paraphrase the original sentence. Original sentence: "a fan film that for the uninitiated plays better on video with the sound turned down" Paraphrased sentence: A fan film that, for those not familiar with the source material, is more enjoyable when watched with the sound turned off. 
Please paraphrase the original sentence. Original sentence: "apparently reassembled from the cutting-room floor of any given daytime soap" Paraphrased sentence: It appears to be pieced together from the outtakes of any given daytime soap opera. 
Please paraphrase the original sentence. Original sentence: "{}" Paraphrased sentence:
\end{shaded}

\noindent
Our paraphrased examples are summarized as follows.

\begin{table}[h]
    \centering
    \begin{tabular}{p{7.3cm}p{7.3cm}}
    \thickhline
        Original & Paraphrased \\ \hline
        a turgid little history lesson , humourless and dull  &
        A dry and tedious history lesson that is devoid of humour or interest.  \\ 
        not so much a movie as a picture book for the big screen .&
        The movie is more of a picture book than a full-fledged movie for the big screen.\\ 
        now it 's just tired .  &
        It is now simply outdated. \\  
    \thickhline
    \end{tabular}
    \caption{Paraphrased examples of SST-5 dataset}
    \label{tab:my_label}
\end{table}

\begin{table}[h]
    \centering
    \begin{tabular}{p{7.3cm}p{7.3cm}}
    \thickhline
        Original & Paraphrased \\ \hline
        for all the wit and hoopla , festival in cannes offers rare insight into the structure of relationships .&
        Festival in Cannes offers rare insight into the structure of relationships.\\ 
        eldom has a movie so closely matched the spirit of a man and his work .&
        A movie seldom has a movie so closely matched the spirit of a man and his work.\\ 
        those of you who are not an eighth grade girl will most likely doze off during this one . &
        8th graders and younger will most likely doze off during this one.\\  
    \thickhline
    \end{tabular}
    \caption{Paraphrased examples of Subj dataset}
    \label{tab:my_label}
\end{table}

\begin{table}[h]
    \centering
    \begin{tabular}{p{7.3cm}p{7.3cm}}
    \thickhline
        Original & Paraphrased \\ \hline
        A friend of mine suggested we go here today before our movie. I was planning on suggesting another place, but she got their early and got a table DARN!I don't hate Red Robin...I think I avoid it because I am not a big fan of hamburgers. Seems like more of a place for straight guys and kids if you ask me, but my experience today wasn't to bad.Our waiter was really nice however I think that may have been a result of my push up bra.Ordered the Crispy Chicken Salad which also had hard boiled egg, bacon, and veggies and was very good. I'll probably get that again next time someone drags me here. Get it with that Italian dressing. Yummy! My friend ordered us onion rings as an appetizer I hate onions, but those were goood! Not my first choice but good crowd pleaser with more decent food than most chains.&
        I was considering going to Red Robin with a friend, but I decided to go somewhere else instead. I was not a big fan of hamburgers, but I was drawn to Red Robin because of the free tastings. I was pleasantly surprised by the friendliness of the staff, especially the waiter who was very attentive and helpful. I ordered the Crispy Chicken Salad, which was very good. I'll probably go back there next time someone drags me there. \\ 
        Huge rooms. Soft towels. Comfortable bed with tons of pillows. Three things that make me happy when I'm traveling. What's wrong with this place, then? First of all, the location is central to nothing aside from the mall which houses several chain restaurants. Second, the staff could not care less about pretty much anything. While the woman who checked us in was helpful and friendly, that was the end of that. Despite requesting my Hilton status "amenities" (just a package of snacks and water...not much), I never received it. I was also charged \$30 for internet when I shouldn't have paid a thing (got the bill corrected at check out). And housekeeping didn't leave enough towels or replace the water. Considering we paid over 200 a night, the blase attitude of the staff is very disappointing. &
        3 things that make me happy when I travel are: spacious rooms, friendly staff, and a comfortable bed with lots of pillows. However, the location is inconvenient, the staff is indifferent, and the amenities are subpar.\\ 
        You can either pay \$5.50 for 3-day movie rentals or get a \$40 membership and pay \$2 for 3-day/\$3 for 7-day rentals. They also offer 2-for-1 movies for students on Tuesday and Thursday. The reason I give 3 stars is because that deal isn't valid for people with memberships!? I learnt this 30 seconds after paying for a membership. I'm a student and could have paid \$2.75 for movies twice a week. Instead I paid \$40 (way too much) for a membership to pay .75 cents less than the other students. Good movie selection and shop but don't fall for their rip off of a membership unless you rent daily. &
        3-day movie rentals cost either \$5.50 or \$40 for a membership. They offer a deal for students on Tuesdays and Thursdays, but it's not valid for those with memberships.\\ 
        
    \thickhline
    \end{tabular}
    \caption{Paraphrased examples of Yelp dataset}
    \label{tab:my_label}
\end{table}
