# Supplementary material for: Distributed In-Context Learning under Non-IID Among Clients
Source: arXiv:2408.00144 source file (2024-07-31)
Supplement: Supplementary file 7 [file 99_prompt_table.tex]

\begin{table}[h]
\centering
\resizebox{0.95\linewidth}{!}{
\begin{tabular}{c|p{3cm}|p{3.1cm}|c|p{6cm}}
\thickhline
Dataset & Prompt & Label & Label Template & Example\\ \hline
AGNews   & Topic of the text: & \{World, Sports, Business, Technology \} & Topic: \textbf{\textit{Label}} & \textcolor{blue}{REDMOND, Wash. - Microsoft Corp. and cable television provider Comcast Corp. said Monday they would begin deploying set-top boxes powered by Microsoft software starting next week. \textbackslash n Topic: Business \textbackslash\textbackslash ...}\textcolor{red}{Oil demand is rising faster than predicted this year as OPEC pumps more low-quality oil in a failed bid to reduce record prices, according to International Energy Agency, an adviser to 26 industrialized nations. \textbackslash n Topic:}  \\ \hline

MR   & Sentiment of the sentence: & \{great, terrible\} & It was \textbf{\textit{Label}} & \textcolor{blue}{"Analyze That" is one of those crass, contrived sequels that not only fails on its own but makes you second-guess your affection for the original. \textbackslash n It was terrible ...}\textcolor{red}{about the only thing to give the movie points for is bravado—to take an entirely stale concept and push it through the audience's meat grinder one more time.\textbackslash n It was }  \\ \hline

SST-5   & Sentiment of the sentence: & \{great, good, okay, bad, terrible\} & It was \textbf{\textit{Label}} & \textcolor{blue}{a strong, funny, and finally transporting re-imagining of Beauty and the Beast and 1930s horror films \textbackslash n It was great ...}\textcolor{red}{no movement, no yuks, not much of anything. \textbackslash n It was}  \\ \hline

Subj   & Subjectivity of the sentence: & \{subjective, objective\} & It's \textbf{\textit{Label}} & \textcolor{blue}{gangs, despite the gravity of its subject matter, is often as fun to watch as a good spaghetti western. \textbackslash n It's subjective ...}\textcolor{red}{smart and alert, Thirteen Conversations About One Thing is a small gem. \textbackslash n It's}  \\ \hline

Amazon    & Sentiment of the sentence: & \{great, good, okay, bad, terrible\} & It was \textbf{\textit{Label}} 
& \textcolor{blue}{Love the originality of this music. Because she is ever-changing, Madonna is never boring. "Music" makes you want to dance - totally energizing! Wish the "Music" video was half as impressive as this work of art. ...}
\textcolor{red}{The case for the DVDs were a bit damaged. The damage did not compromise the DVDs, ... \textbackslash n It's}  \\ \hline

Yelp   & Subjectivity of the sentence: & \{subjective, objective\} & It's \textbf{\textit{Label}} & \textcolor{blue}{My family visited ceasars palace and ate here. Our waiting time was only ten minutes despite all the people. Our server was the best. He recommended several great dishes. The food was higher than our expections....}\textcolor{red}{his place is great. The staff is really friendly and the chile verde burrito is fantastic. You know a ...  \textbackslash n It's}  \\ \hline

Yahoo   & Topic of the sentence & \{Society \& Culture, Science \& Mathematics, Health, Education \& Reference, Computers \& Internet, Sports, Business \& Finance, Entertainment \& Music, Family \& Relationships, Politics \& Government\} & It's \textbf{\textit{Label}} & \textcolor{blue}{who sang message in a bottle? Answer: Sting (the Police) ...}\textcolor{red}{Neuroscience Question? Answer: no it is callef motor neuroprostheses. \textbackslash n Topic: }  \\
\thickhline
\end{tabular}}
\caption{Prompt and instructions used for each dataset. We denote \textcolor{blue}{examples} in blue and \textcolor{red}{queries} in red.}
\label{tab:prompt}
\end{table}
